# Supplementary material for: Superconductivity from a melted insulator
Source: arXiv:2210.06508 source file (2022-10-12)
Supplement: Supplementary file 1 [file supplement.pdf]

# Superconductivity from a melted insulator

S. Mukhopadhyay,[1,*] J. Senior,[1,*] J. Saez-Mollejo,[1] D. Puglia,[1] M. Zemlicka,[1] J. Fink,[1] and A.P. Higginbotham[1,†]
[1] *IST Austria, Am Campus 1, 3400 Klosterneuburg, Austria*

## CONTENTS

I. Extraction of chain parameters 2
A. Josephson energy interpolation 3
B. Chain and junction parameters 3

II. Schematic of the chip 5

III. Device setup and connections 6

IV. Nanofabrication 8

V. Current-peak spacings 8

VI. Base electron temperature 9

VII. Comparing energy scales 10

VIII. Systematics in measurement/analysis 11
A. Heating 11
B. Upturn 12
C. Voltage Offsets 13
D. Power law fits 14
E. Global superfluid stiffness 15

IX. Additional analysis 16
A. Scaling 16
B. Planckian limit 17

X. Theory 18
A. Boundaries in theoretical phase diagram 18

* Equal contribution
† andrew.higginbotham@ist.ac.at

## I. EXTRACTION OF CHAIN PARAMETERS

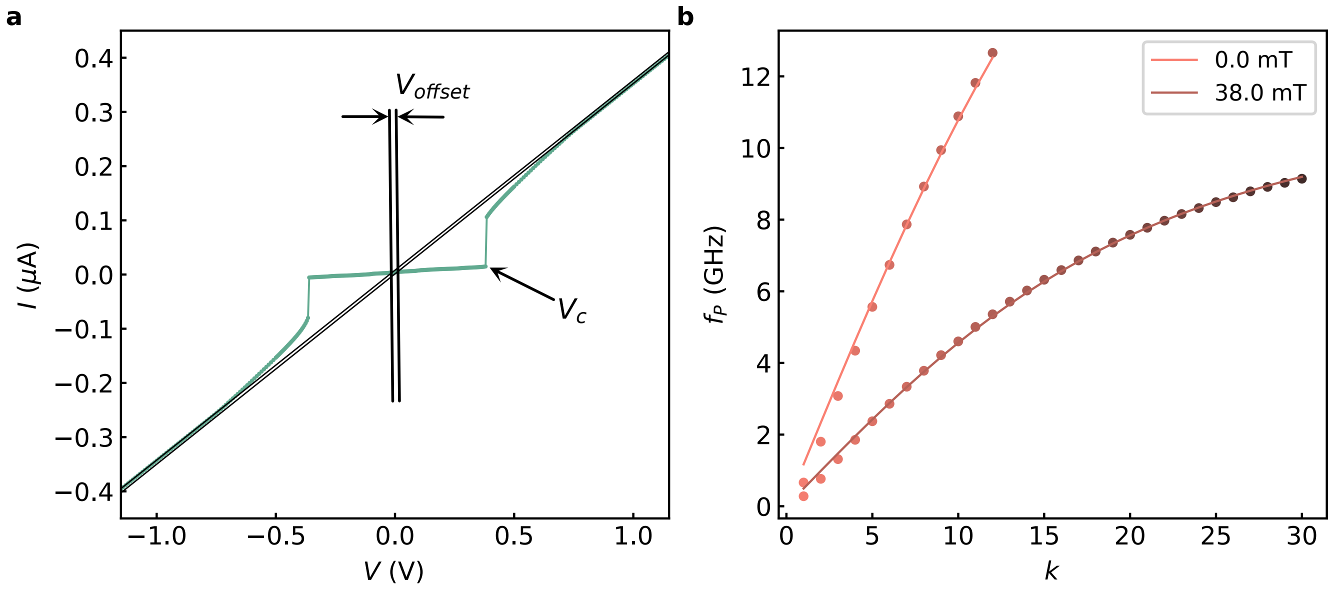


**Figure S1: Extraction of chain parameters $\mathbf{E_C, E_J, E_g}$. a,** Measured current $I$ versus applied voltage $V$. Linear fits to the high bias features extract $E_C, E_J$. $V_c$ is the critical voltage. **b,** Extracted resonant peak frequency $f_P$ versus mode number $k$. The curves are fit from the dispersion relation, which yields $E_g$, and $E_J$ as a function of magnetic field.

In the transport device, a voltage offset $V_{\text{offset}}$ is extracted by extrapolating the linear parts of the current-voltage characteristic down to zero bias (Fig. S1a). $E_C$ is then inferred from $V_{\text{offset}}$ using [15]

$$E_C = 4eV_{\text{offset}}/N, \tag{S1}$$

which gives the value quoted in the main text.

Once $E_C$ is fixed from transport, microwave measurements are used to determine $E_g$ and $E_J(B)$. The dispersion relation for plasma-mode resonant frequency $f_{P,k}$ is

$$f_{P,k} = \omega(k)/\sqrt{1 + (\omega(k)/\omega_p)^2}, \tag{S2}$$

where $\omega_p = \sqrt{2E_J E_C}$ and $\omega(k) = \pi k \sqrt{2E_J E_g}/N$, with $N$ being the number of junctions. Fitting Eq. S2 to the experimental data, as in Fig. S1b, yields $E_g$ and $E_J(B)$. Sample values determined with this method are presented in Fig. S2 and Table SII.

Two independent checks are available on the extracted system parameters. The charging energy $E_C$ can be estimated from geometry and the nominal specific capacitance of our Josephson junctions. Josephson energy can be estimated with the Ambegaokar-Baratoff relation [37]

$$E_J = N\Delta h/(8e^2 R_N), \tag{S3}$$

where $N$ is the number of junctions and $\Delta$ is the superconducting gap of Aluminum. These independent checks on $E_C$ and $E_J$ are shown in Table SIII.

### A. Josephson energy interpolation

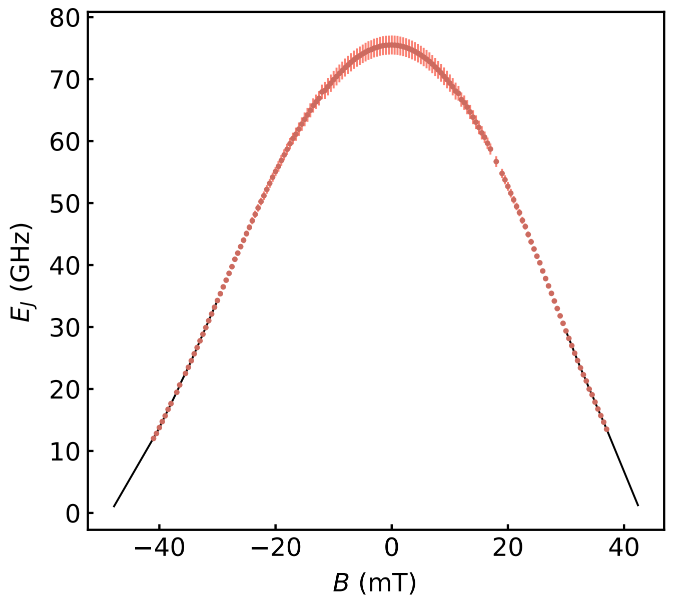


**Figure S2: $\mathbf{E_J(B)}$ interpolation.** Josephson energy $E_J$, determined from fitting dispersion curves, as a function of the magnetic field $B$. Error bars are the standard error resulting from the fits. Black lines represent a linear interpolating function used at higher magnetic fields used to estimate $B^{\text{ins}}$, see Sec. VII for further details.

The field-driven superconductor-insulator transition in our system is expected to occur at a magnetic field $B^{\text{ins}}$. As discussed in Sec. VII, $B^{\text{ins}}$ is determined by numerically solving $\pi K_c(B^{\text{ins}}) = 1$. To accomplish this we interpolate $E_J(B)$ linearly out to $B^{\text{ins}}$, which is justified by the smooth, linear behavior observed in $E_J$ over similar field ranges, as shown in Fig. S2.

### B. Chain and junction parameters

| Parameter | Notation | Microwave | Transport |
|---|---|---|---|
| Number of junctions | $N$ | 1227 | 1217 |
| Chain length | $L$ | 912 $\mu$m | 905 $\mu$m |
| Junction Area | $A$ | $0.28 \pm 0.01$ $\mu$m$^2$ | |

**Table SI: Chain and junction geometry.** Chain length and number of junctions refer to the designed values. Geometry of a junction (or the chain) is estimated from SEM imaging. For details refer to section *Nanofabrication*.

The error in $A$ is the propagated error from estimating length and breadth of a single junction from a SEM image.

| Parameter (@ $B = 0$ T) | Notation | Value | Method |
|---|---|---|---|
| Charging energy | $E_C/h$ | $5.11 \pm 0.04$ GHz | Eq. S1 |
| Charging energy to ground | $E_g/h$ | $1390 \pm 40$ GHz | Fig. S1b |
| Josephson energy | $E_J/h$ | $75.5 \pm 1.5$ GHz | Fig. S1b |
| Normal state resistance of chain | $R_N$ | $2857.11 \pm 0.08$ k$\Omega$ | Fig. S1a |
| Critical voltage of chain | $V_c$ | $0.374 \pm 0.001$ V | Fig. S1a |

**Table SII: Extracted parameters.** For calculations discussed in text, $E_J$ and $E_g$ inferred from microwave measurements are used, whereas $E_C$ inferred from transport measurements are used.

The error in $E_g$ is the standard error in the values of $E_g$ inferred from fits to the dispersion curves at high magnetic

fields. The error in $E_J$ is the standard error from fit to the dispersion curve at B = 0 T. The error in $E_C$, $R_N$ and $V_c$ is the difference between charging energies, high-bias resistances and critical voltages inferred from up and down I-V sweeps.

The following table serves as a cross-check of the junction parameters mentioned in Table SII above:

| **Parameter** | **Value** | **Method** |
|---|---|---|
| Charging energy | $6.1 \pm 0.2$ GHz | $(2e)^2/(2C_s \times A)/h$ |
| Josephson energy | 54.73 $\pm 0.06$ GHz | Eq. S3 |

**Table SIII: Independent checks on extracted parameters.** Empirical specific capacitance of a junction $C_s = 45$ fF/$\mu$m$^2$ [38]. Superconducting gap of bulk Aluminum, $\Delta = 180$ $\mu$eV.

The errors in the parameters of Table SIII are propagated from the errors in $A$ (Table SI) and $R_N$ (Table SII). Table SIV contains a list of chain/junction parameters that have been derived from the measured values presented in Table SII:

| **Parameter (@ $B = 0$ T)** | **Notation** | **Value** | **Formula** |
|---|---|---|---|
| Junction capacitance | $C_c$ | 15.1 $\pm$ 0.1 fF | $(2e)^2/(2E_C)$ |
| Junction capacitance to ground | $C_g$ | 55.9 $\pm$ 1.5 aF | $(2e)^2/(2E_g)$ |
| Junction inductance | $L_J$ | 42.7 $\pm$ 0.8 nH | $(h/2e)^2/(2E_J)$ |
| Impedance | $Z$ | 27.6 $\pm$ 0.6 k$\Omega$ | $\sqrt{L_J/C_g}$ |
| Local superfluid stiffness | $K_C$ | $2.72 \pm 0.04$ | $\sqrt{E_J/2E_C}$ |
| Global superfluid stiffness | $K_g$ | 0.165 $\pm$ 0.003 | $\sqrt{E_J/2E_g}$ |
| Plasma frequency | $\omega_p$ | 27.7 $\pm$ 0.3 GHz | $\sqrt{2E_JE_C}/h$ |
| Charge screening length | $\Lambda$ | 16.4 $\pm$ 0.2 | $\sqrt{E_g/E_C}$ |
| Bloch bandwidth | $W$ | 149 $\pm$ 3 Hz | Eq. S4 |

**Table SIV:** Chain/junction parameters inferred from Table SII.

$$W = 16(E_JE_C/\pi)^{1/2}(2E_J/E_C)^{1/4}e^{-\sqrt{32E_J/E_C}}. \tag{S4}$$

The errors for each parameter in Table SIV are propagated from corresponding errors in the parameters mentioned in Table SII.

## II. SCHEMATIC OF THE CHIP

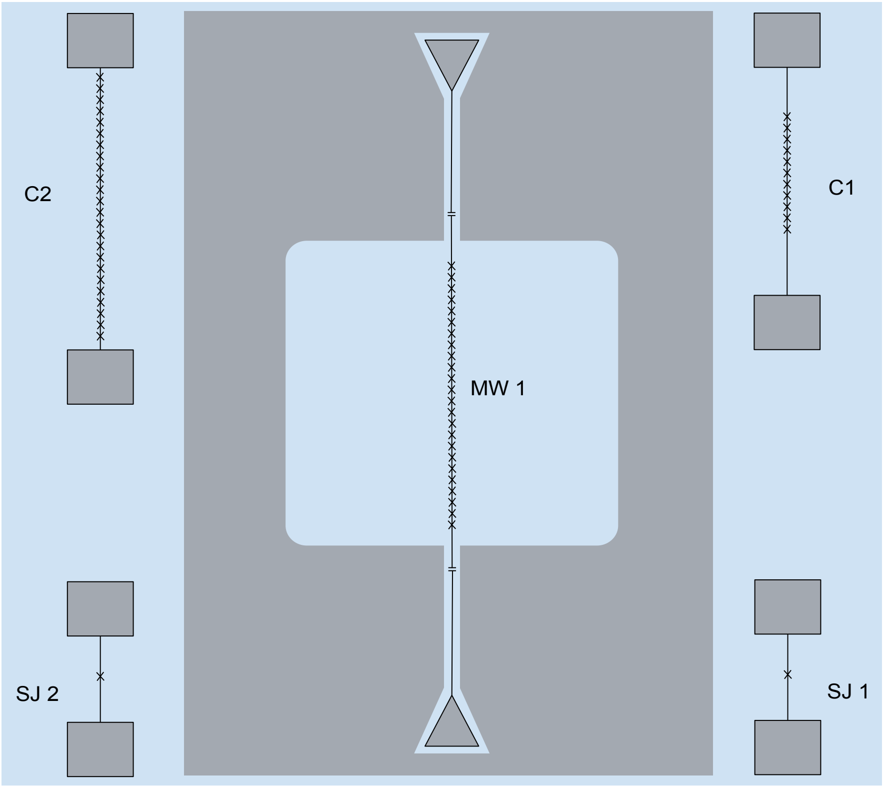


**Figure S3: Schematic of the nanofabricated chip.** Blue background represents Silicon. Grey represents Aluminum. Each cross represents a single Josephson junction.

MW1 refers to the chain of Josephson junctions capacitively coupled on either side to 50 Ω microwave launchers. C1 and C2 refer to transport chains. C2 contains nominally the same number of junctions as on the microwave chain, MW1. C1 has half as many junctions as C2. SJ1 and SJ2 are identical single junction transport devices, with the same junction geometry as on the microwave and transport chain devices. Ground plane around the array of junctions of the microwave device (MW1) has been removed with the intention of decreasing capacitance to ground.

## III. DEVICE SETUP AND CONNECTIONS

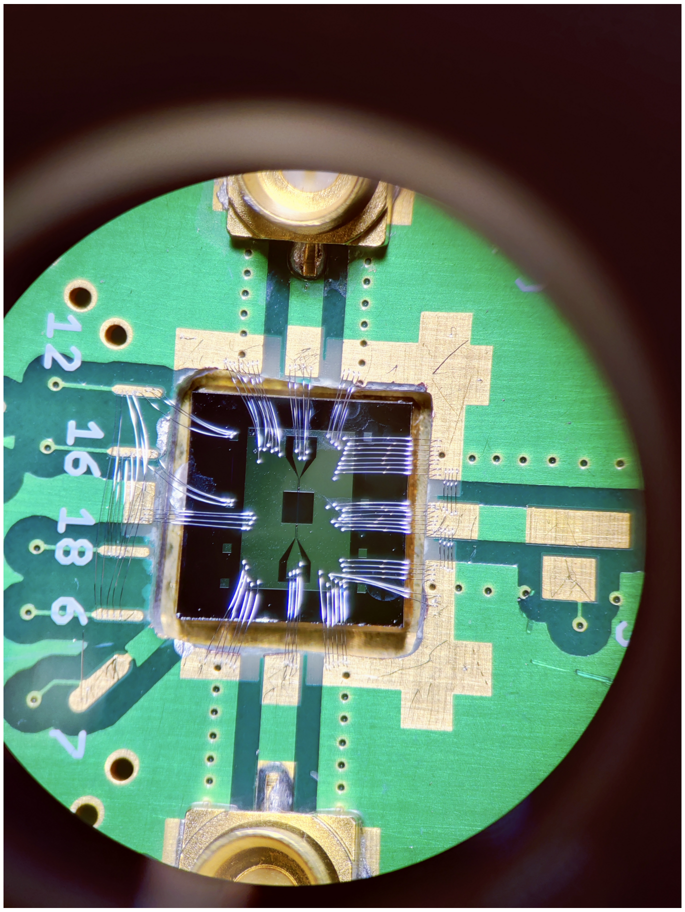


**Figure S4: Chip bonded onto PCB.** Numbers on the PCB indicate connections to DC lines for four/two probe transport measurements. SMP launchers for microwave connections can be seen partially at the top and bottom of the picture.

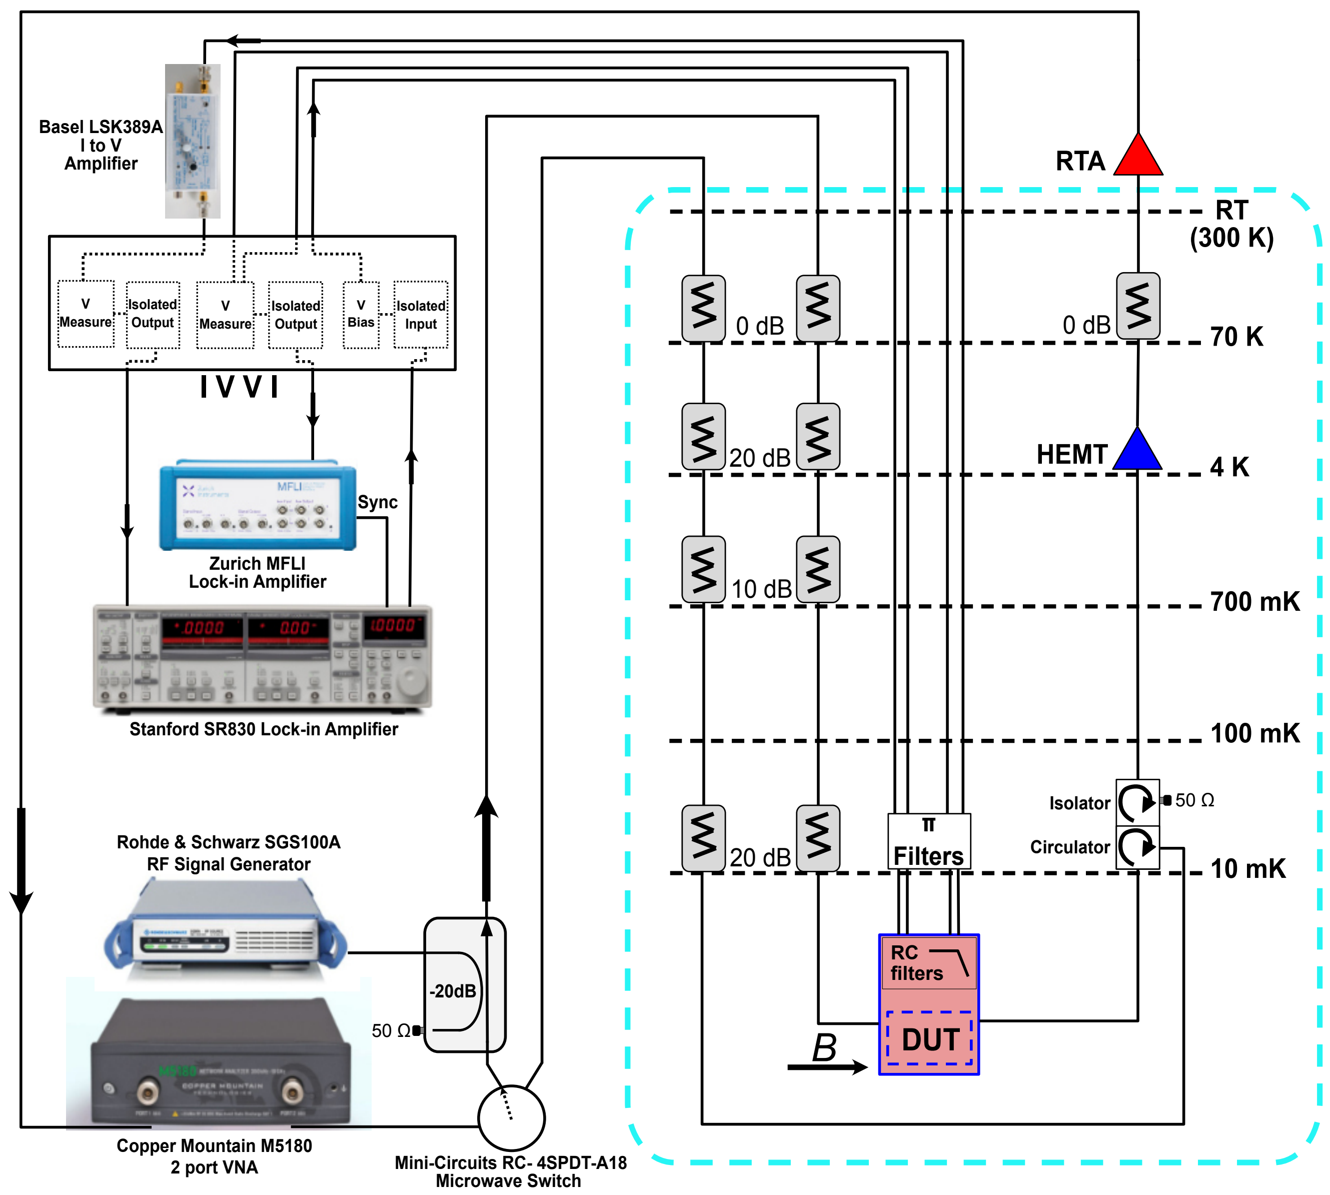


**Figure S5: The experimental setup.** The Dilution Fridge represented as cyan colored dashed boundary. The signal generator is coupled to the output port of the VNA through a RF coupler which has a 20 dB insertion loss at the coupled port. The 'resistor' symbol at each stage of the fridge represent the installed microwave cryogenic attenuators. 'RTA' refers to Room Temperature Amplifier with a gain of around 35 dB. 'HEMT' refers to High-Electron-Mobility-Transistor, which is the Low Noise Amplifier (noise $\sim 2$ K) with a gain of around 36 dB at 4 K. 'DUT' refers to 'Device Under Test'. 'B' indicates the direction of applied external magnetic field.

Microwave measurements are done in transmission, where the output (amplifier) line has double junction isolator attached to the mixing chamber stage of the dilution fridge. In addition, the output line has LNF HEMT attached to the 4 K stage and and another LNF amplifier attached to the room temperature stage of the cryostat. The input line has 50 dB of net attenuation with 0 dB at 70 K stage, 20 dB at 4 K stage, 10 dB at 700 mK stage and 20 dB at mixing chamber stage of the cryostat.

The DC lines are equipped with three cascaded LFCN filter boards attached to the mixing chamber stage of the dilution fridge; each filter board provides cut-off at different frequencies. The three cut-off frequency ranges are (DC – 5000 MHz), (DC – 1450 MHz) and (DC – 80 MHz). Each board has filters soldered onto them in six stages for all the DC lines. The PCB onto which the chip is bonded, has single stage low pass filtering (2 kΩ ; 47 nF) for each DC line. So, in all each DC line has nineteen stage low-pass filtering at the mixing chamber stage of the cryostat.

## IV. NANOFABRICATION

- The chains were fabricated on a high resistivity Silicon substrate ($> 10^4$ Ωcm), which was diced into $7 \times 7$ mm chips, ultrasonicated in Acetone (2 min / power 4) and then in IPA (2 min / power 4).
- The chips were baked at 170 C for 3 mins before spin coating with MMA (EL-13), followed by PMMA (950k 4%). Spin coating recipe was developed such that thickness of MMA is 670 nm and of PMMA is 290 nm. The chips were again baked at 170 C for 3 mins after each spin coating step.
- Standard e-beam lithography was done in Raith EBPG5150, after which the pattern was developed in IPA : water (3 : 1) solution for 90 secs.
- The developed chip was then subjected to electron beam evaporation with Aluminum, in a double angle shadow evaporation process in Plassys UHV MEB550S2, with an intermediate in-situ static oxidation step (5 mbar/5 mins). The evaporation was terminated with another in-situ static oxidation step (10 mbar/2 mins). Before evaporating Aluminum, the evaporation chamber was gettered with Titanium for 3 mins at 0.2 nm/sec to further bring down the pressure of the chamber. In the first evaporation step, 60 nm of Aluminum was deposited, whereas on the second step 120 nm of Aluminum was deposited; with an evaporation rate of 1 nm/sec in both steps.
- Lift-off was done using hot NMP (80 C) for 45 mins, after which the chip was successively cleaned in cold NMP, Acetone and IPA.
- SEM imaging of the JJ chain revealed the junction (or chain) width $\sim$ 510 nm, and the junction overlap $\sim$ 560 nm.

## V. CURRENT-PEAK SPACINGS

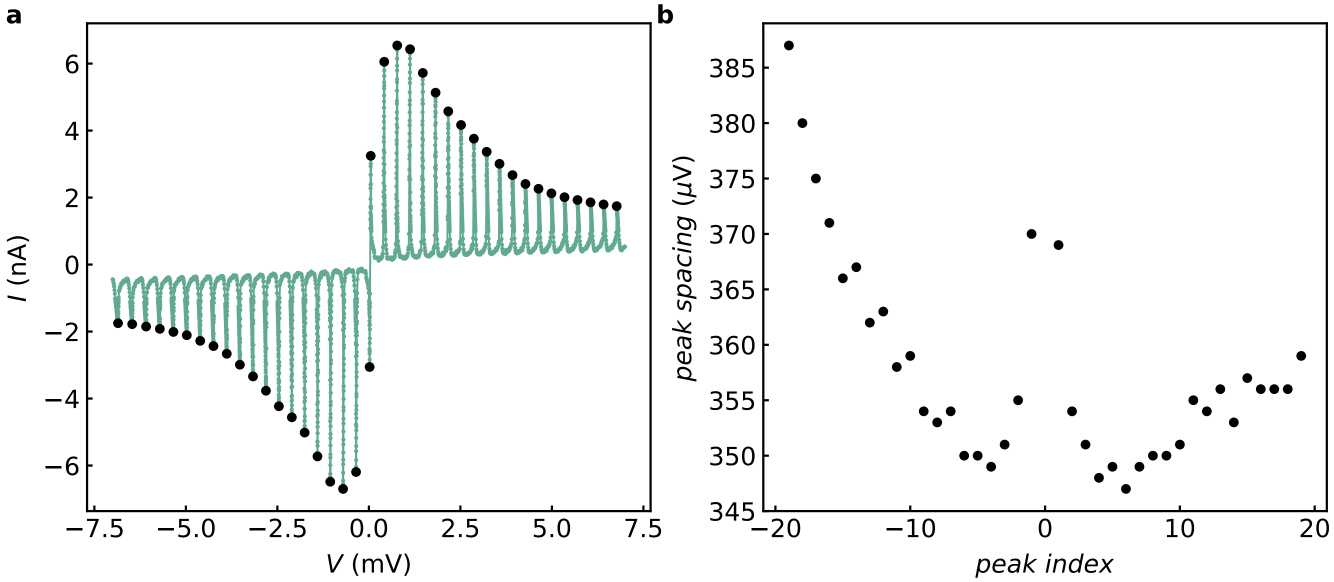


**Figure S6: Peak extraction and spacings. a,** Measured current $I$ versus applied voltage $V$. The black dots represent detected current peaks. **b,** Peak spacings versus the peak index. Each peak index refer to the succeeding peak spacing on positive bias and to the preceding peak spacing on negative bias.

The typical peak spacing is comparable to twice the superconducting gap of Aluminum, 360 $\mu$eV. There is an overall smooth evolution of the peak spacings which is asymmetric in bias, which is not understood (Fig. S6b). Peak spacings are enhanced around zero bias, which we speculate is due to an interaction effect. Namely, the weakest link in the chain is the one which, due to offset charge disorder, is in the deepest Coulomb blockade. This link should switch first, and then require increased bias before current can flow. This picture predicts a that peak spacings should increase near zero bias, as we consistently observe.

## VI. BASE ELECTRON TEMPERATURE

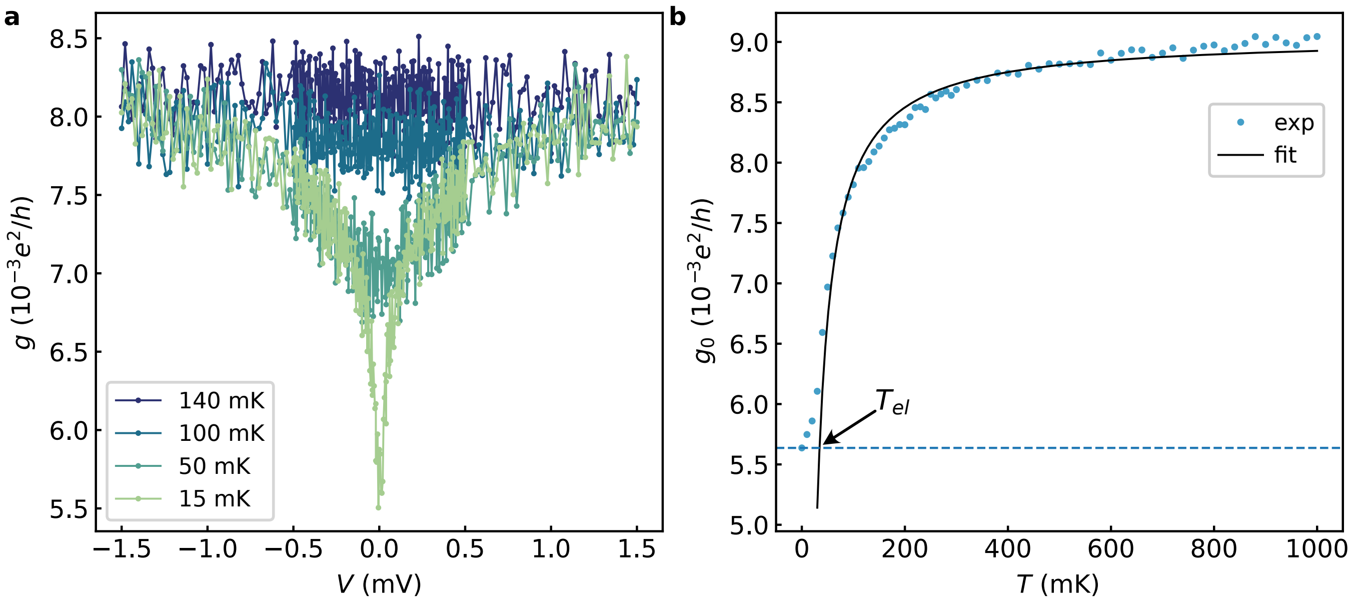


**Figure S7: Coulomb Blockade Thermometry at large magnetic fields. a,** Differential conductance $g$ versus the applied voltage $V$, at various setpoint temperatures. **b,** Zero bias differential conductance $g_0$ versus the setpoint temperature $T$. Black line is a function fit to the data. The dashed blue line is the $g_0$ value corresponding to the lowest data point. $T_{\mathrm{el}}$ is the inferred base electron temperature of the system. Data in this figure is taken with the JJ chain being in normal state, at 500 mT.

Coulomb-blockade thermometry is performed in the normal state by applying a large, perpendicular magnetic field. Measuring differential conductance versus applied voltage shows a sharp dip at zero bias, which gets shallower on raising the temperature of the system (Fig. S7a). Extracting the zero bias differential conductance $g_0$ at all setpoint temperatures, shows a gradual decline in conductance below 400 mK, and a sharp fall below 100 mK (Fig. S7b). $g_0$ is fit to the well-known expression for Coulomb blockade thermometry [44, 45]

$$g_0 = g_T(1 - ((N-1)/N)E_C/(3k_BT)), \tag{S5}$$

where $g_T$ is the asymptotic $g$ at high bias voltages, $N$ is the number of junctions in the chain and $E_C$ is the charging energy of a junction. At high temperature the data agree well with Eq. S5. At low temperature the conductance is larger than the expected value, indicating that the device falls out of equilibrium with the cryostat. Associating the smallest observed conductance with a temperature gives the base electron temperature $T_{\mathrm{el}} = 35$ mK.

## VII. COMPARING ENERGY SCALES

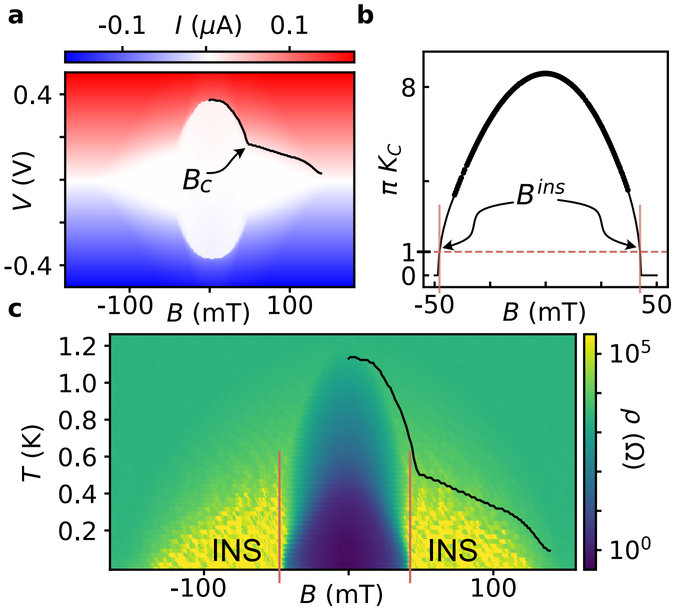


**Figure S8: Overlay of energy scales on the phase diagram. a,** Measured current $I$ versus the bias voltage $V$ and magnetic field $B$. The black curve indicates extracted critical voltage $V_c$. Kink in $V_c$ at critical field $B_c$ indicated. **b,** Inferred local superfluid stiffness $\pi K_C$ versus the magnetic field $B$. Black dots are the inferred stiffness from experimental data. Solid black line is based on a linear extrapolation of $E_J(B)$ down to $E_J \to 0$, which is justified by the empirical observation that $E_J$ is linear at high fields. $B^{\rm ins}$ is defined implicitly by $\pi K_C(B^{\rm ins}) = 1$. **c,** The phase diagram with the zero bias differential specific resistance $\rho$ as a function of the magnetic field $B$ and temperature $T$. INS refers to Insulator. The black curve is the edge feature extracted from **a**, scaled by an empirical proportionality constant of $1/(N2\pi k_B)$. The vertical red lines in **b** and **c** correspond to the field values $|B| = B^{\rm ins}$. Note that, $|B^{\rm ins}| < |B_c|$.

In the main text, we discussed that the wide-range current-voltage characteristic exhibits strongly suppressed current for biases below the critical voltage $V_c$ (Fig. 1b and Fig. S1a). This voltage roughly corresponds to the value for biasing $N$ junctions by $2\Delta/e$ such that current can flow in the voltage state.

Examining the field dependence of this current-voltage characteristic yields further information on the evolution of $\Delta$. Measuring current while varying bias voltage and magnetic field (Fig. S8a) reveals that $V_c$ has a smooth field dependence up to a critical field value of $B_c = 49$ mT, at which point it exhibits a kink. The kink is most likely due to the critical field of the thicker islands in the Josephson array; this is expected critical field for a 120 nm Al film thickness, and also naturally explains why the kink occurs at approximately $V_c(B = 0)/2$. Importantly, this critical field exceeds the field at which insulating behavior is observed $B_c > B^{\rm ins}$, so all islands are superconducting when the array transitions to insulating behavior.

The expected value of $B^{\rm ins}$ is found from the criteria $\pi K_C(B^{\rm ins}) = 1$ (Fig. S8b), yielding a value $B^{\rm ins} = 42.5$ mT at positive field and $B^{\rm ins} = -47.8$ mT at negative field. Since $B^{\rm ins}$ lies slightly beyond the range where microwave measurements are possible, we have performed a linear extrapolation of $E_J(B)$ down to the regime $E_J \to 0$, justified by the linear behavior of $E_J$ over a wide field range. The observed field-asymmetry in $B^{\rm ins}$ reflects the fact that the magnetic-field dependence of the microwave is not perfectly field-symmetric, which is not understood. A consistent field-asymmetry is also present in the transport phase diagram, where the transition to the insulating state is also slightly field-asymmetric. We also note again that $|B_c| > |B^{\rm ins}|$.

As shown in Fig. S8c and also discussed in the main text, the theoretical value of $B^{\rm ins}$ matches the experimentally observed transition to insulating behavior. It is also interesting to note that the overall dependence of $V_c(B)$ qualitatively matches the dome and wing structure of the phase diagram (Fig. S8c, black line).

## VIII. SYSTEMATICS IN MEASUREMENT/ANALYSIS

The zero bias differential resistance of the transport JJ chain was measured using four probe lock-in setup. Stanford SR830 was used to measure the differential current $dI$ through the chain, before which the current signal was converted to voltage using Basel LSK389A transimpedance amplifier. The differential voltage drop across the chain, $dV$ was measured with a Zurich MFLI. A voltage amplitude of 1 $\mu$V was applied, which we experimentally verified was sufficiently small to avoid overheating (see below). Throughout the main text, the two-probe resistance is plotted with the inferred line resistance from a four-probe measurement subtracted. This procedure removes technical noise at the expense of introducing a small (few Ohm) systematic error in the data.

### A. Heating

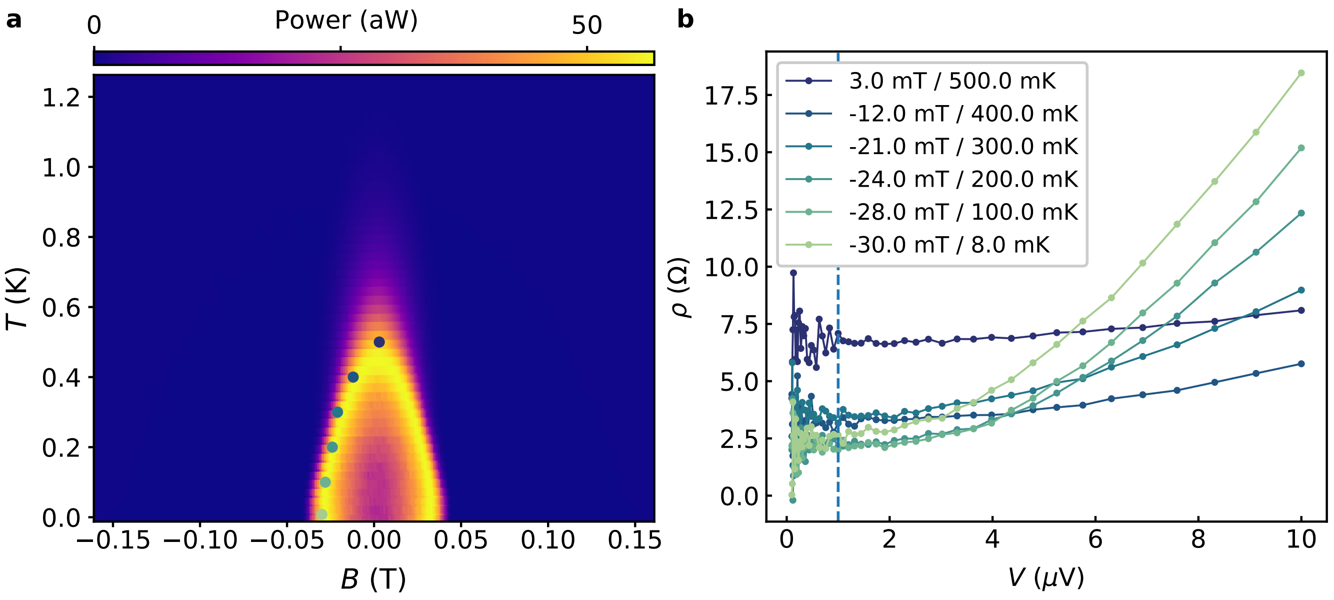


**Figure S9: Heat check for the transport JJ chain. a,** Power dissipated at the chain versus temperature $T$ and magnetic field $B$. **b,** Zero bias differential specific resistance $\rho$ versus lock-in voltage amplitude $V$: at various $(B, T)$ points along the region of maximal power dissipation in **a**. The dashed line indicates the voltage (1 $\mu$V) used for measuring the phase diagram.

Mapping out power dissipated ($dI \times dV$) at the device over full (B,T) parameter space (Fig. S9a), reveals a dome-like feature of maximal power dissipation. Choosing a few points over the dome to do an amplitude study (Fig. S9b), reveals that the device lies comfortably in the linear response regime till 2 $\mu$V of voltage amplitude.

## B. Upturn

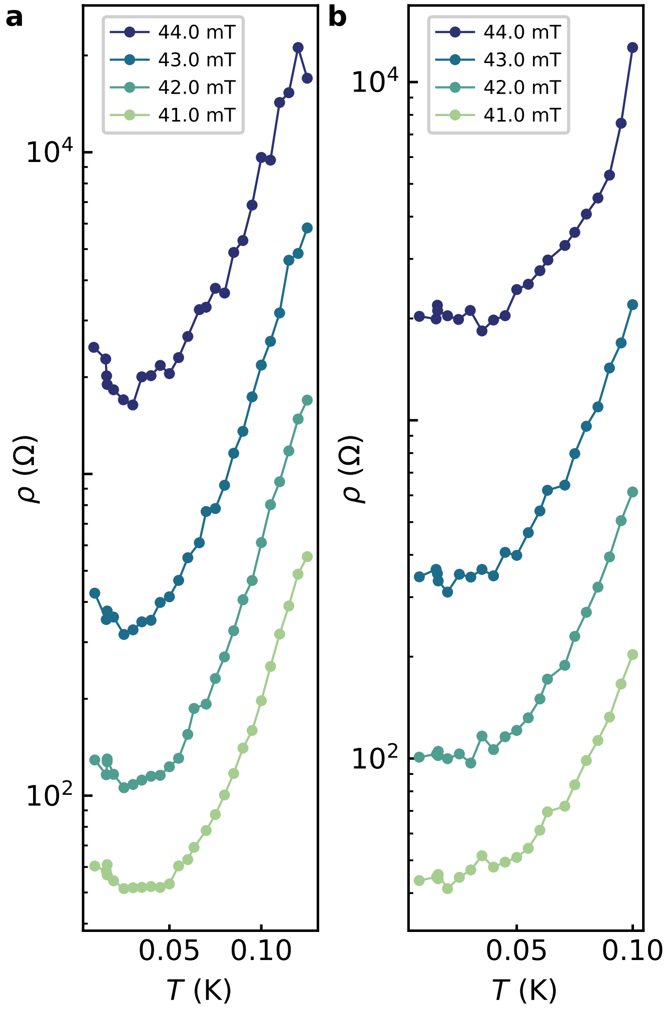


**Figure S10: Reproducibility of the upturn feature. a,** Zero-bias differential specific resistance $\rho$ as a function of measured temperature T, at various magnetic fields. **b,** The same measurement repeated on a different run and same cooldown.

As pointed out in Fig. S10, a low-temperature upturn in resistance is inconsistently observed at fields slightly lower than the data in the main text. The upturn measurement is done at the boundary of LSC/INS phases (refer to Fig. 4c in main text), where on lowering temperature, the device resistance transitions from low to a very high value. Measuring extremely low currents at such phase boundary is challenging, owing to the highly fluctuating values of the locked-in signal. Two customizations were done in this regard:
(a) Turning up the voltage amplitude to 10 $\mu$V.
(b) Measuring the $dI$, $dV$ over ten time points and recording the mean value.
To ensure that the device does not heat up on increasing the lock-in excitation, amplitude study (similar to one depicted in Fig. S9b) was done at temperature corresponding to the minimum resistance. At such regime, the device resistance is higher than the line resistance in the measurement chain, making the device effectively voltage biased. Hence, maximum heating is expected at the point of minimum resistance. However, the device maintained linear response in the amplitude study.

### C. Voltage Offsets

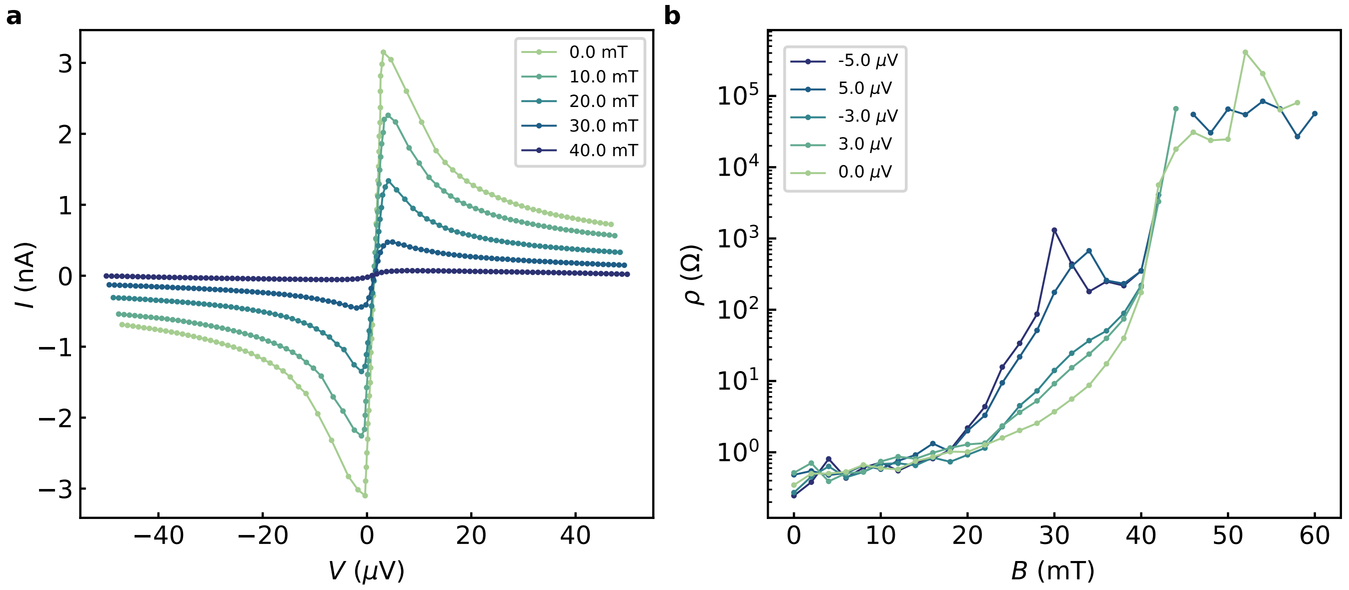


**Figure S11: Effect of voltage offsets in specific resistance measurement. a,** Current $I$ versus the applied voltage $V$, in the narrow bias range, measured at various magnetic fields. **b,** Zero bias specific differential resistance $\rho$ versus the magnetic field $B$, with and without applied offset voltages.

The supercurrent peak, and the zero bias conductance, gradually decreases on increasing the magnetic field (Fig. S11a). Lock-in setup measures the slope of the zero bias peak. As shown in Fig. S11b, adding voltage offsets to the lock-in measurement changes the behavior of the device in the region where the device transitions from LSC to INS phase (refer to Fig. 4c in main text). Hence, ensuring proper offset correction at zero voltage bias is essential to measurement of the phase diagram.

### D. Power law fits

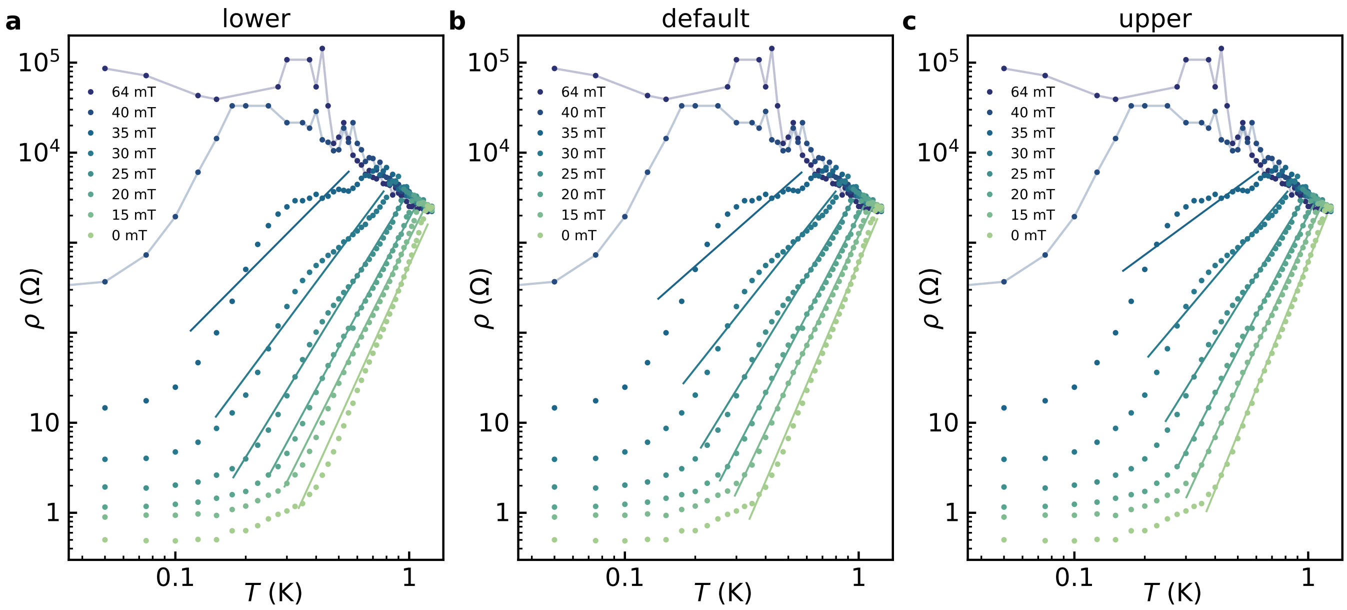


**Figure S12: Power law fits with various choices of lower cutoffs. a,** Zero bias specific differential resistance $\rho$ versus temperature $T$, with 0.18 $T_P$ as the lower cutoff temperature for power law fits. **b,** Same plot with 0.215 $T_P$ as the lower cutoff temperature for fits. **c,** Same plot with 0.25 $T_P$ as the lower cutoff temperature for fits. $T_P$ is the plasma frequency in temperature units.

To analyze the power-law behavior of $\rho(T)$, fits must be performed over a restricted temperature range. Because system parameters evolve with magnetic field, the fit range must also be field dependent. The high-temperature limit of the fitting range is chosen to be 95% of the plasma temperature $T_P$, where

$$T_{\rm p} = \sqrt{2E_J(B)E_C}/k_B. \quad \text{(S6)}$$

As shown in the main text, the upper edge of the local superconducting dome follows the plasma temperature, so this is a suitable upper bound.

The low-temperature limit of the fitting range is not as easy to sharply define, due to the smooth crossover to saturating resistance. To account for this difficulty, we explored a range of lower cutoff values, as shown in Fig. S12. These cutoff values are used to create the blue error bands for the exponent $p$ in Fig. 3b of the main text. To evaluate the impact of the systematic error bands on fit parameters, $p(K_c)$ was fit to a line for the three lower cutoffs in Fig. S12. The range of values obtained are reported as uncertainties in the slope and intercept in the main text.

### E. Global superfluid stiffness

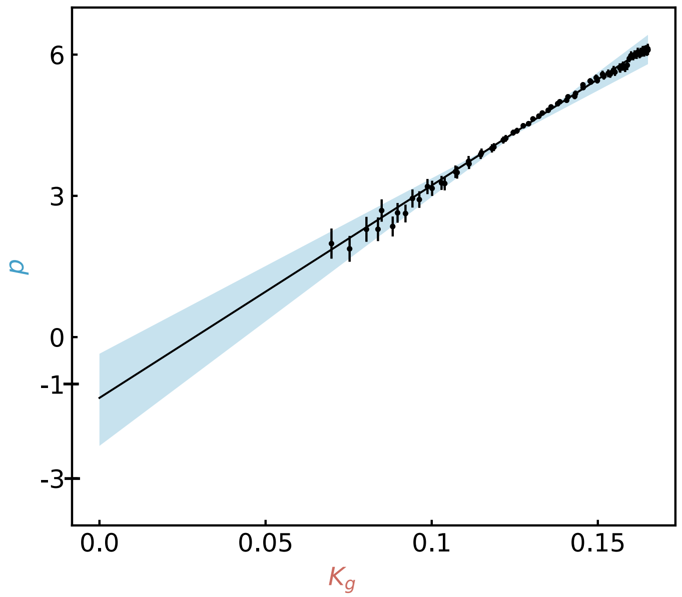


**Figure S13: Comparing the powers with global superfluid stiffness.** Exponent $p$ from power-law fits versus the global superfluid stiffness $K_g$ from microwave measurements. Solid line is a linear fit. Shaded blue region depicts the systematic error resulting from the choice of lower resistance cutoff in the power law fits.

Solving the Renormalization Group (RG) equations in the UV limit, yields a power law with exponent $\pi K_C - 1$ (Eq. S10), where $K_C$ is the bare value of $K$ in RG flow. While solving in the IR limit, with renormalized $K$, results in a power law with exponent $2\pi K_g - 3$.

Comparing $p$ from the transport measurements with the global superfluid stiffness $K_g$ inferred from microwave measurements reveals a linear behavior (Fig. S13) with slope $45 \pm 7$ and intercept of $-1.3 \pm 1.0$. This in complete disagreement with the predicted slope of $2\pi$ for global superconductivity. The intercept close to $-1$ is same as observed for local superconductivity (Fig. 3b in main text), owing to the fact that only the x-axis is scaled down on plotting versus $K_g$.

## IX. ADDITIONAL ANALYSIS

### A. Scaling

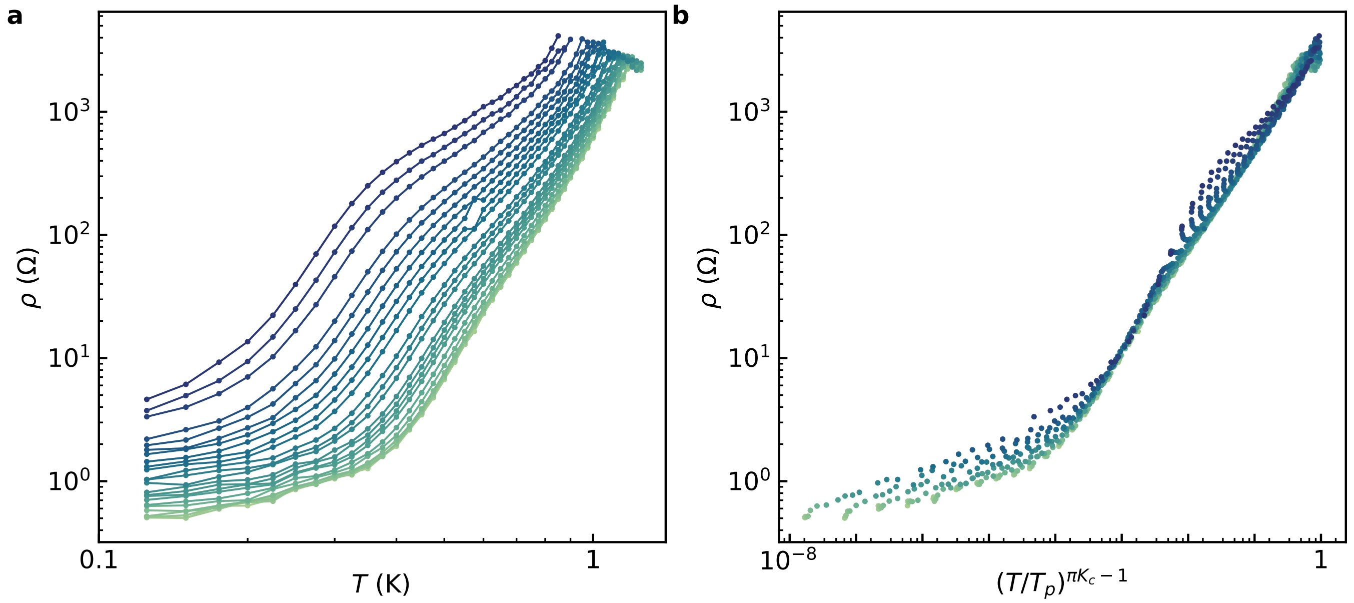


**Figure S14: Collapse of power laws. a,** Zero bias specific differential resistance $\rho$ as a function of temperature $T$, at various magnetic fields. **b,** The same data in **a** plotted with scaled temperature axis, where $T_P$ is the plasma frequency in temperature units and $K_C$ is the local superfluid stiffness.

As shown in Fig. S14a, the power law behavior of specific resistance with temperature is observed until about 40 mT. In Fig. S14b, scaling the normalized temperature axis with expected exponent collapses all the data on left into an universal power law behavior, removing the field dependency of the data. As pointed out earlier in Eq. S6, $T_P$ is a field dependent quantity.

## B. Planckian limit

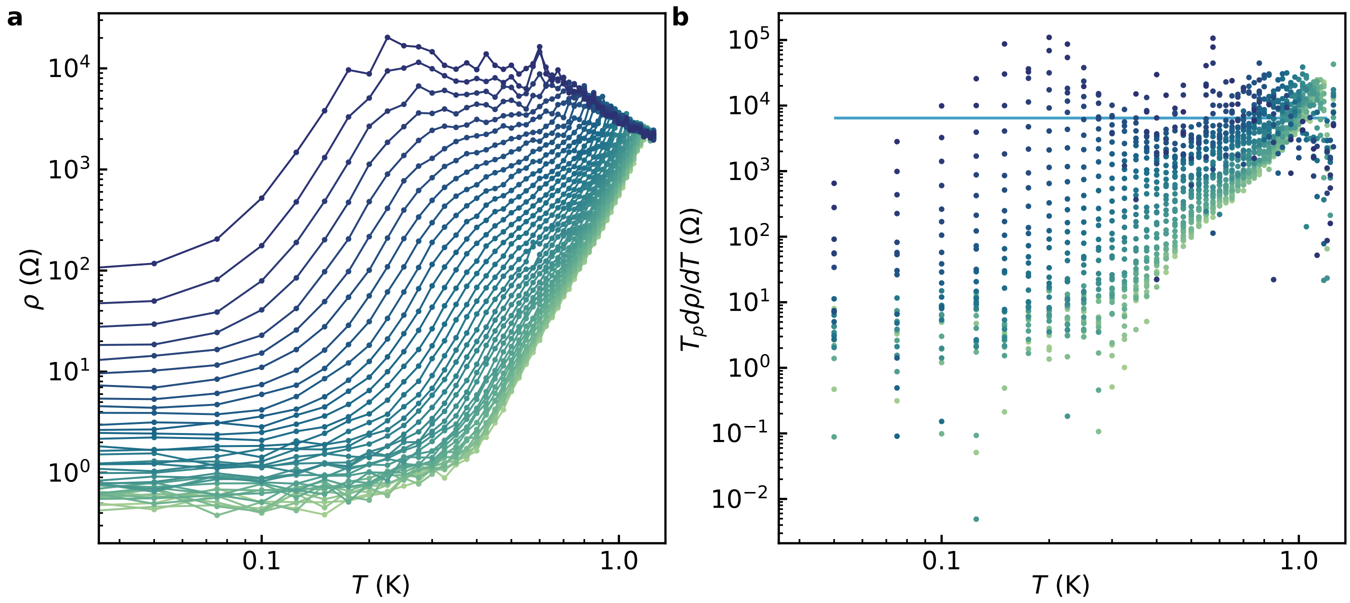


**Figure S15: Planckian slope check. a,** Zero bias specific differential resistance $\rho$ as a function of temperature $T$, at various magnetic fields. **b,** The slope of the curves in **a**, times the plasma frequency $\mathrm{T_P}$, versus temperature $T$. The blue horizontal line is the resistance quantum, $R_Q$.

Our picture for local superconductivity connects the timescale of thermal fluctuations near quantum criticality, $\tau = h/(k_B T)$, to specific resistance. In the literature there is a widely hypothesized connection between the Planckian scattering time $\tau_s = h/(k_B T)$ and quantum-critical metals [39–43]. Given recent reports of Planckian scattering in a superconductor-insulator system [36], and of the qualitative similarity of some of our specific resistance curves to Ref. [36], we were motivated to directly compare our data with a model of Planckian scattering. Following the method of Ref. [36], we computed $T_P d\rho/dT$, where the plasma temperature $T_P$ plays the role of the high-temperature cutoff for superconducting behavior in our system. The Planckian bound is $T_P \cdot d\rho/dT < h/(4e^2)$. As shown in Fig. S15b, the observed resistance exceeds this bound by more than an order of magnitude. Thus, the Planckian bound apparently does not apply in our system.

## X. THEORY

Here we give an overview of the theoretical origin of power-law scaling discussed in the main text.

The key simplification for our case arises from the fact that the dimensionless phase slip fugacity, $y \propto e^{-4\sqrt{2E_J/E_C}}$ is small, less than $10^{-10}$ at zero magnetic field. This allows us to work with linearized renormalization group equations from Ref. [13], which in the long-screening-length limit ($\Lambda \gg 1$) takes the form

$$\frac{dK}{dl} = -K(1-u_g) \tag{S7}$$

$$\frac{du_g}{dl} = 2u_g(1-u_g) \tag{S8}$$

$$\frac{dy}{dl} = \frac{1+u_g}{2}(2-\pi K)y. \tag{S9}$$

Here $K$ is the superfluid stiffness, taking the initial value $K_C = \sqrt{E_J/2E_C}$ and $u_g$ takes the initial value $1/(1+\Lambda^2)$, where $\Lambda$ is the charge screening length, representing the plasmon group velocity in the UV limit in units of the plasma frequency. Following Ref. [13], we assume the renormalization flow is terminated at the thermal length given by $e^l = \Omega_\mathrm{p}/T$ where $\Omega_\mathrm{p} = \sqrt{2E_J E_C}$ is the single junction plasma frequency. The resistance is then given by $R = R_0 y^2/e^l$.

Equations (S7-S8) express the renormalization of $K$ from its ultraviolet value of $K_C$ down to $K_g$ at the fixed point $u_g = 1$.

In the high temperature limit where $K$ is hardly renormalized, resistance follows the power law behavior

$$R = R_0 \left(\frac{T}{\Omega_\mathrm{p}}\right)^{\pi K_C - 1}. \tag{S10}$$

At lower temperature $K$ is renormalized down and the system crosses over to insulating behavior. The crossover temperature depends on system parameters,

$$T_\mathrm{ins} = \max(2E_C/\pi, \sqrt{2E_J E_C}/\Lambda). \tag{S11}$$

The first case occurs in the limit of small Josephson energy, and insulating behavior appears because $K$ is renormalized below $1/\pi$, at which point the system enters strong coupling. The second case occurs in the limit of large Josephson energy, and insulating behavior appears because the system crosses over to the infrared limit where $u_g = 1$, which is the case we focus on in the main text.

In the experiment, the two terms in Eq. S11 are actually comparable, so it is perhaps surprising that a square-root behavior is observed in Fig. 4a of the main text. As we caution in the main text, the experimentally extracted $T^*$ may not map directly on to $T_\mathrm{ins}$, and indeed different metrics give different quantitative behavior.

### A. Boundaries in theoretical phase diagram

The superconductor-insulator transition is strictly only a phase transition at $T = 0$; otherwise it is a crossover [2]. The theoretical phase diagram in the main text in fact labels crossover boundaries, where the temperature dependence of the specific resistance $d\rho/dT$ changes sign. To identify these points, we work perturbatively in the limit of small phase-slip fugacity, as discussed above.

At low temperatures where the infrared fixed-point of Eqs. (S7-S8) is reached, the $\rho(T)$ power law is $2\pi K_g - 3$, which gives the low-temperature crossover $\pi K_g \sim 3/2$. Note that once terms of order $y^2$ are included into Eq. S9, one would actually find either the Giamarchi-Schulz or BKT fixed points depending on if disorder is included [2, 23]. Since this correction is small compared to those associated with local superconductivity discussed in the main text, we simply indicate the crossover point with a $\sim$ to avoid ambiguity.

By similar logic, in the high-temperature limit $\rho(T)$ power law is $\pi K_C - 1$, which yields the local superconductor-insulator crossover $\pi K_C \sim 1$.

The boundary between local and global regimes is given by Eq. S11, which when smoothly interpolated yields the theoretical diagram in the main text.
